# Supplementary material for: Topological Dynamical Decoupling
Source: arXiv:1909.10697 source file (2019-09-24)
Supplement: Supplementary file 1 [file supplemental.pdf]

# Supplemental Materials for Topological Dynamical Decoupling

Jiang Zhang,[1,2] Xiao-Dong Yu,[3] Gui-Lu Long,[1,4,5,2,*] and Qi-Kun Xue[1,5,2,†]

[1] *State Key Laboratory of Low-Dimensional Quantum Physics and Department of Physics, Tsinghua University, Beijing 100084, China*
[2] *Beijing Academy of Quantum Information Sciences, Beijing 100193, China*
[3] *Naturwissenschaftlich-Technische Fakultät, Universität Siegen, Walter-Flex-Straße 3, 57068 Siegen, Germany*
[4] *Beijing National Research Center for Information Science and Technology, Beijing 100084, China*
[5] *Collaborative Innovation Center of Quantum Matter, Beijing 100084, China*

## I. A FORMAL DEFINITION OF GROUP $\mathcal{B}^1$

To formalize our idea, the square lattice's vertices, edges and faces are renamed as 0-cells (labeled as $v$), 1-cells ($e$) and 2-cells ($f$), respectively [1]. The sets of $i$-cells ($i = 0, 1, 2$) are labeled as $\mathcal{V} = \{v_k\}$, $\mathcal{E} = \{e_k\}$, and $\mathcal{F} = \{f_k\}$, respectively, where $k$ is the element index. Accordingly, a subset of $\mathcal{V}$ ($\mathcal{E}$ or $\mathcal{F}$) is labeled as $\mathcal{V}'$ ($\mathcal{E}'$ or $\mathcal{F}'$). For the set of $i$-cells, all its subsets form an Abelian group $\mathcal{C}^i$ with the addition as the group operation and the empty set being the identity element. This idea can be formalized by introducing the concept of $i$-chains, each of which is related to a subset of $i$-cells. Without loss of generality, we take 2-cells as an example. For a subset $\mathcal{F}'$, its corresponding 2-chain can be defined as

$$c_i^2 = \sum_k c_k f_k, \quad c_k = \begin{cases} 0, & f_k \notin \mathcal{F}'; \\ 1, & f_k \in \mathcal{F}', \end{cases} \tag{S1}$$

where $c_i^2$ is the $i$-th element of group $\mathcal{C}^2$. The 2-chains can be added together to obtain another 2-chain by taking into account the addition rule $f_k + f_k = 0$ which gives rise to the Abelian structure of group $\mathcal{C}^2$. Similarly, we can form the Abelian groups $\mathcal{C}^0$ and $\mathcal{C}^1$ with the rules $v_k + v_k = 0$ and $e_k + e_k = 0$, respectively.

Next, we introduce a boundary operator $\partial^2$ which acts on the 2-chains by the following way:

$$\partial^2 : \mathcal{C}^2 \to \mathcal{C}^1, \tag{S2}$$

i.e., $\partial^2$ takes 2-chains to their boundaries which are 1-chains. For example, the face $f_1$ [see Fig. 1(a)] has the set of edges $\{e_1^u, e_1^d, e_1^l, e_1^r\}$ as its boundary [$e_1^i$ ($i = u, d, l, r$) are the up, down, left, and right edges for $f_1$, respectively], then $\partial^2 f_1 = e_1^u + e_1^d + e_1^l + e_1^r$. The boundary operator $\partial^2$ acts on a 2-chain $c_i^2 = f_1 + f_2 + \cdots + f_m$ as $\partial^2 c_i^2 = \partial^2 f_1 + \partial_2 f_2 + \cdots + \partial_2 f_m$.

Based on the operator $\partial^2$, we can define a group $\mathcal{B}^1$ as a subgroup of $\mathcal{C}^1$. $\mathcal{B}^1$ contains all the images of $\partial^2$ from $\mathcal{C}^2$. This means that an element of $\mathcal{B}^1$ is the boundary of a 2-chain, $b = \partial^2 c^2$ ($b \in \mathcal{B}^1$ and $c^2 \in \mathcal{C}^2$). Thus, the 1-chain $e_1^u + e_1^d + e_1^l + e_1^r$ is an element of $\mathcal{B}^1$ since it is the boundary of $f_1$. Some group elements of $\mathcal{B}^1$ are illustrated in Fig. 1.

Consider a periodic square lattice with $n$ rows and $n$ columns [see Fig. 1(a)]. Each element of $\mathcal{B}^1$ is the boundary of a 2-chain which contains one or more squares in the lattice. When a 2-chain has only one square, e.g., $f_k$ in Fig. 1(a), its boundary is the 1-chain which consists the four edges surrounding it. The corresponding element can be written as

$$\partial^2 f_k = e_k^u + e_k^d + e_k^l + e_k^r, \tag{S3}$$

where $e_k^i$ ($i = u, d, l, r$) are the upper, down, left, and right edges for $f_k$, respectively. When a 2-chain has two separate squares, e.g., $f_1$ and $f_2$, its boundary contains eight edges,

$$\partial^2(f_1 + f_2) = \sum_{i=1,2} e_i^u + e_i^d + e_i^l + e_i^r. \tag{S4}$$

On the other hand, when two squares in a 2-chain are adjacent, e.g., $f_3$ and $f_4$ in Fig. 1(a), they share a common edge. The corresponding boundary can be written as

$$\partial^2(f_3 + f_4) = e_3^u + e_3^l + e_3^r + e_4^d + e_4^l + e_4^r, \tag{S5}$$

where $e_3^d = e_4^u$ is the common edge and has been cancelled according to the addition rule $e_3^d + e_4^u = 0$ [see Fig. 1(b)]. A special case arises when a set of squares forms a row or column in the lattice. For example, six squares (from $f_5$ to

$f_{10}$) in Fig. 1(a) construct a row in the lattice. In this case, the related group element is the 1-chain including only the upper and lower edges of each square, reading

$$\partial^2(\sum_{i=5}^{10} f_i) = \sum_{j=5}^{10} e_j^u + e_j^d. \tag{S6}$$

Moreover, according to the addition rule, every element of $\mathcal{B}^1$ is the inverse element of itself. This also indicates that the empty set 0 is the identity element of $\mathcal{B}^1$.

## II. THE FIRST HOMOLOGY GROUP

To see the topological nature of group $\mathcal{B}^1$, we define another boundary operator $\partial^1$ which acts on the 1-chains by the following way:

$$\partial^1 : \mathcal{C}^1 \to \mathcal{C}^0, \tag{S7}$$

i.e., $\partial^1$ takes 1-chains to their boundaries which are 0-chains constituted by vertices. Since each edge on a square lattice has two endpoints (vertices), we have $\partial^1 e_k = v_k^1 + v_k^2$. Accordingly, if we have a 1-chain $c = e_1 + e_2 + \cdots + e_m$, then $\partial^1 c = \partial^1 e_1 + \partial^1 e_2 + \cdots + \partial^1 e_m$. Based on $\partial^1$, we can define a group $\mathcal{Z}^1$ which is another subgroup of $\mathcal{C}^1$. The elements of $\mathcal{Z}^1$ are the 1-chains that have no boundary, i.e., $\partial^1 z = 0$ ($z \in \mathcal{Z}^1$). Geometrically, $\mathcal{Z}^1$ is the set of closed curves in the lattice. The crucial observation here is that all boundaries of 2-chains are also closed curves,

$$\partial^1 \circ \partial^2 c = 0, \forall c \in \mathcal{C}^2. \tag{S8}$$

It follows that $\mathcal{B}^1$ is a subgroup of $\mathcal{Z}^1$ ($\mathcal{B}^1 \subset \mathcal{Z}^1$).

Actually, $\mathcal{B}^1$ is an invariant subgroup of $\mathcal{Z}^1$. Thus, we can define the first homology group as the quotient group of $\mathcal{Z}^1$ and $\mathcal{B}^1$,

$$\mathcal{H}^1 \equiv \mathcal{Z}^1/\mathcal{B}^1. \tag{S9}$$

It is worthy to notice that, although we consider a particular lattice here, the group $\mathcal{H}^1$ only depends on the topology of the surface since all the information about the lattice has been removed by taking the quotient [2]. In fact, for a surface with genus $G = k$, $\mathcal{H}^1 \simeq \mathbf{Z}_2^{2k}$. This result has direct applications to surface codes [3], which is one of the promising quantum error correction approaches for fault-tolerant quantum computation. More exactly, if the square lattice is attached on a surface with genus $k$, the first homology group provides a topology degree of $2^{2k}$, which allows the encoding of $2k$ logical qubits.

## III. REALIZING THE DECOUPLING PROCEDURE $D^z$ WITH EULERIAN CYCLES

The evolution operator generated by $H_t$ (the Hamiltonian for the total system) can be written as

$$U_t(t) = \mathrm{T}\exp\{-i\int_0^t H_t(s)\mathrm{d}s\} \tag{S10}$$

where T is the time-ordering operator, and $\hbar$ is taken to be 1 hereafter. On the other hand, the evolution operator generated by the control Hamiltonian can be written as

$$U_c(t) = \exp\{-i\int_0^t H_c^z(s)\mathrm{d}s\}, \tag{S11}$$

where $H_c^z(s)$ is a piecewise constant Hamiltonian constructed with $H_1^z$ and $H_2^z$. By performing the transformation that removes the control Hamiltonian, the dynamics of the total system is governed by the time-dependent Hamiltonian

$$H(t) = U_c^\dagger(t) H_t(t) U_c. \tag{S12}$$

Correspondingly, the overall evolution operator in the Schrödinger picture takes the form

$$U(t) = U_c(t)\mathrm{T}\exp\{-i\int_0^t H(s)\mathrm{d}s\}. \tag{S13}$$

When $U_c(t)$ is cyclic [i.e., $U_c(t+T_c)=U_c(t)$ for a period $T_c$], the instantaneous evolution operator at time $T=mT_c$ ($m$ is an integer) can be written as

$$U(T)=\exp\{-i\bar{H}T\}, \tag{S14}$$

where $\bar{H}$ can be calculated with Magnus expansion. In particular, the first order of $\bar{H}$ can be written as

$$\bar{H}^0=\frac{1}{T_c}\int_0^{T_c}H(t)\mathrm{d}t. \tag{S15}$$

To realize $D^z$ with bounded-strength controls, we choose an Eulerian cycle [4] which can be written as

$$I\xrightarrow{t_1}t_1\xrightarrow{t_2}t_{12}\xrightarrow{t_1}t_2\xrightarrow{t_2}I\xrightarrow{t_2}t_2\xrightarrow{t_1}t_{12}\xrightarrow{t_2}t_1\xrightarrow{t_1}I. \tag{S16}$$

The corresponding control Hamiltonian reads

$$H_c(t)=\begin{cases}H_1^z & 0\le t<\tau\\ H_2^z & \tau\le t<2\tau\\ H_1^z & 2\tau\le t<3\tau\\ H_2^z & 3\tau\le t<4\tau\\ H_1^z & 4\tau\le t<5\tau\\ H_2^z & 5\tau\le t<6\tau\\ H_1^z & 6\tau\le t<7\tau\\ H_2^z & 7\tau\le t<8\tau\end{cases}, \tag{S17}$$

where $H_i^z=\frac{\pi}{2\tau}\sum_{k\in S_i}\sigma_z^k$ with $\tau$ being the time interval for a step and $S_i$ being the set of qubits related with $t_i$. Accordingly, the control evolution operator can be written as

$$U_c(t)=\begin{cases}e^{-iH_z^1t}, & 0\le t\le\tau;\\ e^{-iH_z^2(t-\tau)}t_1, & \tau\le t<2\tau;\\ e^{-iH_z^1(t-2\tau)}t_2t_1, & 2\tau\le t<3\tau;\\ e^{-iH_z^2(t-3\tau)}t_2, & 3\tau\le t<4\tau;\\ e^{-iH_z^1(t-4\tau)}, & 4\tau\le t<5\tau;\\ e^{-iH_z^2(t-5\tau)}t_1, & 5\tau\le t<6\tau;\\ e^{-iH_z^1(t-6\tau)}t_2t_1, & 6\tau\le t<7\tau;\\ e^{-iH_z^2(t-7\tau)}t_2, & 7\tau\le t<8\tau\end{cases}. \tag{S18}$$

Substituting Eq. (S17) and Eq. (S18) into Eq. (S15), we obtain the effective Hamiltonian $H_{D^z}^E$:

$$H_{D^z}^E=\bar{H}^0=\frac{1}{8\tau}\sum_{k=0}^{3}g_k^\dagger[\sum_{l=1}^{2}\int_0^\tau e^{iH_z^lt}H_{SE}e^{-iH_z^lt}\mathrm{d}t]g_k=H_{D^z}, \tag{S19}$$

where $g_0=I$, $g_1=t_1$, $g_2=t_2$, and $g_3=t_1t_2$.

## IV. BUILDING LOGICAL OPERATORS WITH MODIFIED EULERIAN CYCLES

The control $U_c(t)$ is implemented by applying $H_c(t)$. However, in the presence of $H_{SE}$, the application of the same control Hamiltonian may result in an actual evolution operator $U(t)$ whose action deviates from the intended one since $H_c(t)$ generally does not commute with $H_{SE}$.

The difference between $U(t)$ and $U_c(t)$ can be described with an operator $\Phi(t)$ [5, 6], i.e.,

$$U(t_2,t_1)=U_c(t_2,t_1)\exp\{-i\Phi(t_2,t_1)\}. \tag{S20}$$

In our case, $H_c(t)$ is chosen to be piecewise, and the time interval $\tau$ for every piece is equal. Therefore, $U_c(t)$ can be separated into pieces according to $H_c$. Explicitly, we denote $U_c(n\tau)$ as

$$U_c(n\tau,0)=U_c(n\tau,(n-1)\tau)\cdots U_c(2\tau,\tau)U_c(\tau,0)=U_c^n\cdots U_c^2U_c^1. \tag{S21}$$

Due to the existence of $H_{SE}$, the real evolution operator can be written as

$$U(n\tau, 0) = U_c(n\tau, 0)\exp\{-i\Phi(n\tau, 0)\}. \tag{S22}$$

The first order of $\Phi(n\tau, 0)$ reads [5, 6],

$$\Phi^0 = \sum_{j=1}^{n} (U_c^{j-1})^\dagger \Phi_j U_c^{j-1}, \tag{S23}$$

where $\Phi_j = \int_{(j-1)\tau}^{j\tau} U_c^\dagger(t) H_{SE} U_c(t) \mathrm{d}t$.

When $H_{SE}$ consists of only $\sigma_x \otimes B_x$ and $\sigma_y \otimes B_y$, we substitute Eq. (S18) into Eq. (S23), and obtain that $\Phi^0 = 0$. This shows that $U_c$ in Eq. (S18) is a concrete example to eliminate the gate errors caused by $H_{SE}$. However, the implementation of $U_c$ performs only the decoupling procedure, leaving the logical qubit unchanged. If we want to build logical gates to the qubits, a modified Eulerian cycle is needed, which can be written as

$$I \xrightarrow{t_1} t_1 \xrightarrow{I} t_1 \xrightarrow{t_2} t_{12} \xrightarrow{I} t_{12} \xrightarrow{t_1} t_2 \xrightarrow{I} t_2 \xrightarrow{t_2} I \xrightarrow{t_2} t_2 \xrightarrow{t_1} t_{12} \xrightarrow{t_2} t_1 \xrightarrow{t_1} I \xrightarrow{U^L} U^L, \tag{S24}$$

where $U^L$ is the intended logical gate. Compared with Eq. (S16), the above cycle comprises four added steps (three identities and one $U^L$). It is easy to show that, if the four steps experience the same error $\Phi_j$, its average will be zero after the group action.

This is possible because the three identities and $U^L$ can be generated by the same Hamiltonian. We take the logical Pauli-$z$ operator as an example. A perfect square lattice on a torus supports two logical qubits. Based on our definition, the logical Pauli-$z$ operators are strings of $\sigma_z^i$ surrounding the "handle" or genus on the lattice, taking the form $\otimes_i \sigma_z^i$. This can be realized with the Hamiltonian

$$H_z^L(t) = \frac{\omega(t)}{2} \sum_{i \in S_z} \sigma_z^i, \tag{S25}$$

where $S_z$ is the set of qubits along the line associated with the logical Pauli-$z$ operator.

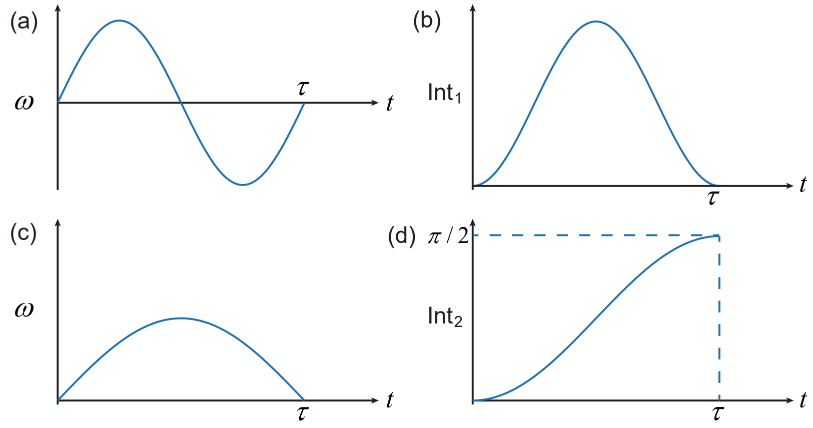


FIG. S1. (a) and (b) are the control profile $\omega(t)$ and its integration $\mathrm{Int}_1$ for implementing the identity, respectively. (c) and (d) are the control profile $\omega(t)$ and its integration $\mathrm{Int}_2$ for implementing the logical operator, respectively.

To realize an identity with $H_z^L(t)$, the profile of $\omega(t)$ can be chosen as shown in Fig. S1(a), where the upward peak and the downward peak are of the same shape but with opposite directions. The corresponding integration $\mathrm{Int}_1(t) = \int_0^t \omega(s)\mathrm{d}s$ is shown in Fig. S1(b). Since $U_I(t) = \exp\{-i\int_0^t H_z^L(s)\mathrm{d}s\}$, it is clear that $U_I(\tau) = I$. On the other hand, $U_z^L$ can be constructed when the profile of $\omega(t)$ is chosen as shown in Fig. S1(c), where $\mathrm{Int}_2(\tau) = \int_0^\tau \omega(t)\mathrm{d}t = \frac{\pi}{2}$ [shown in Fig. S1(d)]. When $\int_0^\tau \mathrm{Int}_1(t)\mathrm{d}t = \int_0^\tau \mathrm{Int}_2(t)\mathrm{d}t$ is satisfied, the error term $\Phi_I$ related to the three identities equals to the error term $\Phi_U$ related to $U_z^L$, because

$$\Phi_I = \int_0^\tau U_I^\dagger(t) H_{SE} U_I(t)\mathrm{d}t = \int_0^\tau U_z^\dagger(t) H_{SE} U_z(t)\mathrm{d}t = \Phi_U, \tag{S26}$$

where $U_z(t) = \exp\{-i\int_0^t H_z^L(s)\mathrm{d}s\}$. The logical Pauli-$x$ operators can be constructed similarly.

## V. REALIZING THE DECOUPLING PROCEDURE $D^{xz}$ WITH EULERIAN CYCLES

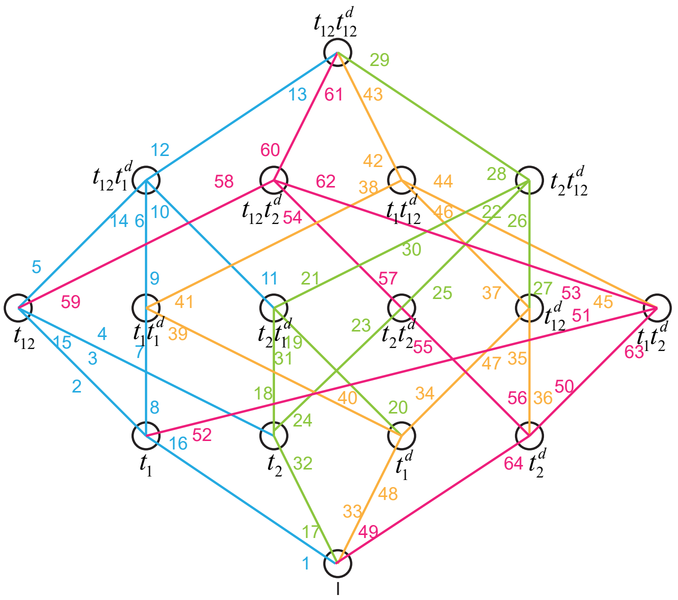


FIG. S2. The Cayley graph and an Eulerian cycle for the group $\mathcal{T}^z \times \mathcal{T}^x$. On the diagram, the circles represent the vertices of the Cayley graph, and the colored lines are the edges for the Eulerian cycles. The Eulerian cycle has 64 edges, each of which connects two vertices (group elements) with a number from 1 to 64, indicating the order of the steps. The blue lines are the edges with numbers from 1 to 16, the pink lines are the edges with numbers from 17 to 32, the yellow lines are the edges with numbers from 33 to 48, and the green lines are the edges with numbers from 49 to 64.

The decoupling procedure $D^{xz}$ involves the decoupling group $\mathcal{T}^z \times \mathcal{T}^x$, which has four generators (i.e., $t_1$, $t_2$, $t_1^d$, and $t_2^d$) and 16 elements. Thus, the corresponding Cayley graph contains 16 vertices, and an Eulerian cycle on this graph consists of 64 edges. We find one Eulerian cycle and illustrate it in Fig. S2. The related control steps are as follows:

$$
\begin{aligned}
& I \xrightarrow{t_z^1} t_z^1 \xrightarrow{t_z^2} t_z^{12} \xrightarrow{t_z^1} t_z^2 \xrightarrow{t_z^1} t_z^{12} \xrightarrow{t_x^1} t_z^{12}t_x^1 \xrightarrow{t_z^2} t_z^1t_x^1 \xrightarrow{t_x^1} t_z^1 \xrightarrow{t_x^1} t_z^1t_x^1 \xrightarrow{t_z^2} t_z^{12}t_x^1 \xrightarrow{t_z^1} t_z^2t_x^1 \\
& \xrightarrow{t_z^1} t_z^{12}t_x^1 \xrightarrow{t_x^2} t_z^{12}t_x^{12} \xrightarrow{t_x^2} t_z^{12}t_x^1 \xrightarrow{t_x^1} t_z^{12} \xrightarrow{t_z^2} t_z^1 \xrightarrow{t_z^1} \\
& I \xrightarrow{t_z^2} t_z^2 \xrightarrow{t_x^1} t_z^2t_x^1 \xrightarrow{t_z^2} t_x^1 \xrightarrow{t_z^2} t_z^2t_x^1 \xrightarrow{t_x^2} t_z^2t_x^{12} \xrightarrow{t_x^1} t_z^2t_x^2 \xrightarrow{t_x^2} t_z^2 \xrightarrow{t_x^2} t_z^2t_x^2 \xrightarrow{t_x^1} t_z^2t_x^{12} \xrightarrow{t_z^2} t_x^{12} \\
& \xrightarrow{t_z^2} t_z^2t_x^{12} \xrightarrow{t_z^1} t_z^{12}t_x^{12} \xrightarrow{t_z^1} t_z^2t_x^{12} \xrightarrow{t_x^2} t_z^2t_x^1 \xrightarrow{t_x^1} t_z^2 \xrightarrow{t_z^2} \\
& I \xrightarrow{t_x^1} t_x^1 \xrightarrow{t_x^2} t_x^{12} \xrightarrow{t_x^1} t_x^2 \xrightarrow{t_x^1} t_x^{12} \xrightarrow{t_z^1} t_z^1t_x^{12} \xrightarrow{t_x^2} t_z^1t_x^1 \xrightarrow{t_z^1} t_x^1 \xrightarrow{t_z^1} t_z^1t_x^1 \xrightarrow{t_x^2} t_z^1t_x^{12} \xrightarrow{t_z^2} t_z^{12}t_x^{12} \\
& \xrightarrow{t_z^2} t_z^1t_x^{12} \xrightarrow{t_x^1} t_z^1t_x^2 \xrightarrow{t_x^1} t_z^1t_x^{12} \xrightarrow{t_z^1} t_x^{12} \xrightarrow{t_x^2} t_x^1 \xrightarrow{t_x^1} \\
& I \xrightarrow{t_x^2} t_x^2 \xrightarrow{t_z^1} t_z^1t_x^2 \xrightarrow{t_x^2} t_z^1 \xrightarrow{t_x^2} t_z^1t_x^2 \xrightarrow{t_z^2} t_z^{12}t_x^2 \xrightarrow{t_z^1} t_z^2t_x^2 \xrightarrow{t_z^2} t_x^2 \xrightarrow{t_z^2} t_z^2t_x^2 \xrightarrow{t_z^1} t_z^{12}t_x^2 \xrightarrow{t_x^2} t_z^{12} \\
& \xrightarrow{t_x^2} t_z^{12}t_x^2 \xrightarrow{t_x^1} t_z^{12}t_x^{12} \xrightarrow{t_x^1} t_z^{12}t_x^2 \xrightarrow{t_z^2} t_z^1t_x^2 \xrightarrow{t_z^1} t_x^2 \xrightarrow{t_x^2} I. \qquad \text{(S27)}
\end{aligned}
$$

## VI. COMBINING WITH CONCATENATED DYNAMICAL DECOUPLINGS

In the main text, our decoupling procedures (such as $D^z$ and $D^{xz}$) have only considered decoherence up to the first order in time. In the ideal case, $H_{SE}$ can be removed from the dynamics of the qubits via periodic DD (i.e., applying a dynamical decoupling procedure periodically). However, in a practical case, higher-order errors may arise due to a finite time interval between two adjacent pulses. In this section, we propose to use the concatenated DD (CDD) to eliminate higher-order errors so that the decoupling procedures $D^z$ and $D^{xz}$ can be used in a long time period.

The basic idea of CDD is to implement a decoupling procedure recursively. For example, when the procedure $D^z = [t_1t_2, \tau, t_1, \tau, t_2t_1, \tau, t_1, \tau, I]$ ($\tau$ is a constant) is relevant, its second-order concatenated form can be written as

$$D^z_2 = [t_1t_2, D^z, t_1, D^z, t_2t_1, D^z, t_1, D^z, I], \tag{S28}$$

which takes a total time of $16\tau$ (assuming the decoupling operators are applied instantaneously). It is clear that, while the first-order error Hamiltonians can be removed by $D^z$, the remaining second-order errors in $D^z$ can be dynamically averaged by $D^z_2$. Similarly, the third-order concatenated form of $D^z$ can be written as

$$D^z_3 = [t_1t_2, D^z_2, t_1, D^z_2, t_2t_1, D^z_2, t_1, D^z_2, I], \tag{S29}$$

which takes a total time of $64\tau$. Higher-order forms can be constructed by following the same way.

On the other hand, the second-order concatenated form of $D^{xz} = [t^d_1t^d_2, D^z, t^d_1, D^z, t^d_2t^d_1, D^z, t^d_1, D^z, I]$ reads

$$\begin{aligned} D^{xz}_2 = [&t^d_1t^d_2t_1t_2, D^z, t_1, D^{xz}, t_2t_1, D^{xz}, t_1, D^{xz}, t^d_1t_1t_2, D^{xz}, t_1, D^{xz}, t_2t_1, D^{xz}, t_1, D^{xz}, \\ &t^d_1t^d_2t_1t_2, D^{xz}, t_1, D^{xz}, t_2t_1, D^{xz}, t_1, D^{xz}, t^d_1t_1t_2, D^{xz}, t_1, D^{xz}, t_2t_1, D^{xz}, t_1, D^{xz}, I], \end{aligned} \tag{S30}$$

and higher-order forms can be obtained similarly. It is worthy to point out that $D^{xz}_2$ requires $64\tau$ to implement the procedure once. Since $64\tau$ must be shorter than the coherence time of the qubits, CDD actually puts a stringent constraint on the time interval $\tau$. Moreover, given the same $\tau$, whether CDD performs better than PDD schemes depends on $\tau$ and the error models.

## VII. REMOVING $H_{SE}$ FROM THE DYNAMICS OF THE QUBITS IN A FINITE SQUARE LATTICE WITH $\mathcal{B}^{z\prime}$ AND $\mathcal{B}^{x\prime}$

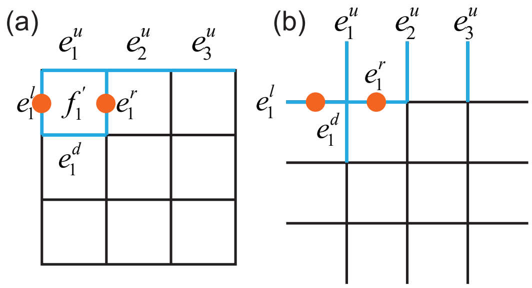


FIG. S3. (a) A $3 \times 3$ finite square lattice. The qubits attached on the edges $e^l_1$ and $e^r_1$ are qubits $a$ and $b$, respectively. (b) The dual lattice of the original lattice in (a).

The main difference between a finite planar lattice and a periodic one is that the former one has boundaries. Thus, unlike the periodic case, there are two kinds of qubits (i.e., edges) attached on a finite planar lattice: those on the edges belonging to the boundaries and those on the edges inside the lattice. A qubit placed on the boundaries relates to only one square while a qubit placed inside the lattice is shared by two adjacent squares.

Now consider a finite planar square lattice with $n$ rows and $n$ columns [see Fig. S3 for an example]. There are a total of $n^2$ squares (labeled by $f'_1, f'_2, \cdots, f'_{n^2}$) and $2(n^2+n)$ edges in the lattice. It follows that the lattice contains $2^{n^2}$ 2-chains, the boundaries of which form a group $\mathcal{B}^{1\prime}$ (as we did for $\mathcal{B}^1$). However, the constraint $\partial^2(\sum_{i=1}^{n^2} f'_i) = 0$ is not valid in this case, implying that the order of group $\mathcal{B}^{1\prime}$ is $2^{n^2}$.

Based on group $\mathcal{B}^{1\prime}$, the first decoupling group $\mathcal{B}^{z\prime}$ can be defined. An element $b^{z\prime}_i \in \mathcal{B}^{z\prime}$ is obtained by replacing each edge of the related element $b^{1\prime}_i \in \mathcal{B}^{1\prime}$ with the $\sigma_z$ operator acting on the associated qubit. To clear up $H_{SE}$ from the dynamics of the qubits, we design a decoupling procedure with $\mathcal{B}^{z\prime}$: $D^{z\prime} = [b^{z\prime}_{2^{n^2}}, \tau, b^{z\prime}_{2^{n^2}} b^{z\prime}_{2^{n^2}-1}, \cdots, b^{z\prime}_3 b^{z\prime}_2, \tau, b^{z\prime}_2 b^{z\prime}_1, \tau, b^{z\prime}_1]$, where $b^{z\prime}_i$ are the group elements of $\mathcal{B}^{z\prime}$ and $\tau$ is the free evolution time.

To see how $\mathcal{B}^{z\prime}$ works, we need to examine the qubits on the boundaries and the qubits inside the lattice separately. For a qubit on the boundaries [e.g., the qubit $a$ attached on $e^l_1$ in Fig. S3(b)], it is related to only one square ($f'_1$). Therefore, among the boundaries of all the $2^{n^2}$ 2-chains, there are $2^{n^2-1}$ boundaries contain $e^l_1$. This indicates that

the corresponding $2^{n^2-1}$ group elements of $\mathcal{B}^{z\prime}$ have $\sigma_z^a$ while the others do not. A group element $b_i^{z\prime}$ which comprises $\sigma_z^a$ transforms $H_{SE}^a = \sigma_x^a \otimes E_x^a + \sigma_y^a \otimes E_y^a + \sigma_z^a \otimes E_z^a$ into

$$b^{z\prime} H_{SE}^a b^{z\prime} = -\sigma_x^a \otimes E_x^a - \sigma_y^a \otimes E_y^a + \sigma_z^a \otimes E_z^a. \tag{S31}$$

On the contrary, the group elements that do not contain $\sigma_z^a$ leave $H_{SE}^a$ unchanged. Thus, the resultant dynamically averaged operator takes the form of

$$\prod_{\mathcal{B}^{z\prime}} (H_{SE}^a) = \sigma_z^a \otimes E_z^a. \tag{S32}$$

On the other hand, the qubits attached inside the lattice (e.g., the qubit $b$ on the edge $e_1^r$) are shared by two adjacent squares. With a similar argument, one can easily show that the corresponding dynamically averaged operator can also be written as

$$\prod_{\mathcal{B}^{z\prime}} (H_{SE}^b) = \sigma_z^b \otimes E_z^b. \tag{S33}$$

Altogether, the decoupling group $\mathcal{B}^{z\prime}$ generates a dynamically averaged operator for $H_{SE}$, reading

$$H_{D^{z\prime}} = \prod_{\mathcal{B}^{z\prime}} (H_{SE}) = \sum_{i=1}^{2n^2+n} \sigma_z^i \otimes E_z^i. \tag{S34}$$

The remaining $H_{D^{z\prime}}$ can be removed by the group $\mathcal{B}^{x\prime}$ defined on the dual lattice of the original finite planar one. Similarly, the dual one is obtained by rotating each edge in the original lattice around its middle point for $\pi/2$. Different from the original lattice, the dual one has $n+1$ rows and $n+1$ columns. This indicates that there are $(n+1)^2$ squares in the dual lattice, but we note that there are $(n-1)^2$ complete squares (those inside the lattice) and $4n$ incomplete squares (those forming the boundaries). The boundary of an incomplete square comprises two (e.g., the square formed by $e_1^l$ and $e_1^u$) or three (e.g., the square formed by $e_1^u$, $e_1^r$, and $e_2^u$) edges.

Again, the boundaries of all the 2-chains in the dual lattice form a group $\mathcal{B}^{1\prime d}$ which has $2^{n^2+2n}$ elements. Further, the second decoupling group $\mathcal{B}^{x\prime}$ can be defined based on $\mathcal{B}^{1\prime d}$ as what we did for $\mathcal{B}^x$. Using $\mathcal{B}^{x\prime}$ as the second decoupling group, we design the decoupling procedure $D^{xz\prime} = [b^{x\prime}_{2n^2+2n}, D^{z\prime}, b^{x\prime}_{2n^2+2n} b^{x\prime}_{2n^2+2n-1}, \cdots, b_3^{x\prime} b_2^{x\prime}, D^{z\prime}, b_2^{x\prime} b_1^{x\prime}, D^{z\prime}, b_1^{x\prime}]$, where $b_i^{x\prime}$ are the elements of group $\mathcal{B}^{x\prime}$. As each qubit in the dual lattice is shared by two squares, a similar argument implies that

$$H_{D^{xz\prime}} = \prod_{\mathcal{B}^{x\prime}} (H_{D^{z\prime}}) = 0, \tag{S35}$$

showing that $H_{SE}$ is completely removed from the dynamics of the qubits on the finite square lattice.

---


* gllong@tsinghua.edu.cn
† qkxue@tsinghua.edu.cn



[1] *Quantum Error Correction*, edited by D. A. Lidar and T. A. Brun (Cambridge University Press, Cambridge, UK, 2013).
[2] J. F. Cornwell, *Group Theory in Physics* (Academic, New York, 1984).
[3] S. B. Bravyi and A. Y. Kitaev, Quantum codes on a lattice with boundary, arXiv:quant-ph/9811052.
[4] L. Viola and E. Knill, Robust Dynamical Decoupling of Quantum Systems with Bounded Controls, Phys. Rev. Lett. **90**, 037901 (2003).
[5] K. Khodjasteh and L. Viola, Dynamically Error-Corrected Gates for Universal Quantum Computation, Phys. Rev. Lett. **102**, 080501 (2009).
[6] K. Khodjasteh and L. Viola, Dynamical quantum error correction of unitary operations with bounded controls, Phys. Rev. A **80**, 032314 (2009).
